# Supplementary material for: Learning Augmented Binary Search Trees
Source: arXiv:2206.12110 source file (2022-06-24)
Supplement: Supplementary file 1 [file Appendix.tex]

\section{Appendix}

\textbf{Proof of \hyperref[thm:ERanCost]{Theorem \ref*{thm:ERanCost}}}
\label{appendix:ERanCost}
\begin{proof}
The expected depth of key $i$ is well known to be $H_i + H_{n-i+1} - 2$ \cite{treaps}. Let $X$ be the depth of an access and let $X_{ij}$ be the depth of key $i$ if it is the $j^{th}$-ranked item, and $0$ otherwise.
\allowdisplaybreaks
\begin{align*}
    E[X] &=\sum_{i = 1}^n \frac{1}{n}\sum_{j = 1}^n  E[X_{ij}] \\
    &=  \sum_{i = 1}^n \frac{1}{n}\sum_{j = 1}^n p_j(H_i + H_{n-i+1} - 2) \\
    &= \sum_{i = 1}^n \frac{1}{n}(H_i + H_{n-i+1} - 2) \\
    &= \frac{2}{n}\sum_{i = 1}^n H_i - 1 \\
    &= \frac{2}{n}((n+1)H_{n+1} - 2n)\\
    &> 2H_{n+1} - 4
\end{align*}
\end{proof}
